# Supplementary material for: A determinantal point process for column subset selection
Source: arXiv:1812.09771 source file (2018-12-23)
Supplement: Supplementary file 1 [file algorithmsappendix.tex]

%!TEX root=./submitted.tex
We recall in this section the algorithms used in the article.

\begin{figure}[!ht]
\centerline{
\scalebox{0.9}{
\begin{algorithm}{$\Algo{DPP}\big(\bm{K})$}
%\vspace{-.1cm}
\Aitem $(\bm{V},\bm{\Lambda}) \longleftarrow \text{eig}(\bm{K})$
\Aitem $Y \longleftarrow  \emptyset$
\Aitem $T \longleftarrow  \emptyset$
\Aitem \For $t \in [d]$
\Aitem \mt Sample $u \sim \mathcal{U}\left[0,1\right]$
\Aitem \mt \If $u \leq \lambda_{t}$
\Aitem \mtt $T \longleftarrow  T \cup \{t\}$
\Aitem $s\bm{V} \longleftarrow  \bm{V}_{:,T}$
\Aitem \While $\text{rk}(s\bm{V}) > 0 $
\Aitem \mt  Sample $i$ from $\Omega$ with probability $\Prb(i) \propto \|s\bm{V}_{i,:}\|_{2}^{2}$
\Aitem \mt  $Y \longleftarrow  Y \cup \{i\}$
\Aitem \mt $\bm{V} \longleftarrow \bm{V}_{\perp}$ an orthonormal basis of $\Span(\bm{V} \cap \bm{e}_{i}^{\perp})$
\Aitem \Return $Y$
\end{algorithm}
}
}
\caption{Pseudocode of sampling from a DPP of marginal kernel $\bm{K}$.}
\label{alg:DPP_SAMPLER}
\end{figure}

\begin{figure}[!ht]
\centerline{
\scalebox{0.9}{
\begin{algorithm}{$\Algo{k-DPP}\big(\bm{L})$}
%\vspace{-.1cm}
\Aitem $(\bm{V},\bm{\Lambda}) \longleftarrow \text{eig}(\bm{L})$
\Aitem $Y \longleftarrow  \emptyset$
\Aitem Sample $T \subset [r], |T| = k$ such that $\Prb(T) \propto \frac{\prod_{i \in T}\lambda_{i}}{\sum\limits_{U \subset[r],|U| = k}\prod_{i \in U}\lambda_{i}}$
\Aitem $s\bm{V} \longleftarrow  \bm{V}_{:,T}$
%$$
\Aitem \While $\text{rk}(s\bm{V}) > 0 $
\Aitem \mt  Sample $i$ from $\Omega$ with probability $\Prb(i) \propto \|s\bm{V}_{i,:}\|_{2}^{2}$
\Aitem \mt  $Y \longleftarrow  Y \cup \{i\}$
\Aitem \mt $\bm{V} \longleftarrow \bm{V}_{\perp}$ an orthonormal basis of $\Span(\bm{V} \cap \bm{e}_{i}^{\perp})$
\Aitem \Return $Y$
\end{algorithm}
}
}
\caption{Pseudocode of sampling from a k-DPP of kernel $\bm{L}$.}
\label{f:kDPP_SAMPLER}
\end{figure}
